# Supplementary material for: An Analysis of Negation in Natural Language Understanding Corpora
Source: arXiv:2203.08929 source file (2022-03-16)
Supplement: Supplementary file 2 [file params_nlu_task_row.tex]

\begin{tabular}{lcccccccc}
\toprule
Hyper-parameters & CmmnsnsQA   & COPA   & QQP    &  STS-B   &  QNLI  &   WiC  & WSC    &  SST-2 \\
\midrule
Max Epochs      &  10    & 50     & 3      &   10     &  3     &   10   &  200   &  3\\
Batch Size      &  16    & 16     & 16     &   16     &  8     &   16   &  16    &  16\\
Learning Rate   &  1e-5  & 1e-5   & 1e-5   &   1e-5   &  1e-5  &   1e-5 &  1e-6  &   1e-5\\
\bottomrule

\end{tabular}
